# Supplementary material for: Zenix: Efficient Execution of Bulky Serverless Applications
Source: arXiv:2206.13444 source file (2024-05-12)
Supplement: Supplementary file 1 [file appendix-main.tex]

\documentclass[letterpaper,twocolumn,10pt]{article}
\usepackage{usenix}

\urlstyle{rm}

\usepackage[numbers,sort,compress]{natbib}

\usepackage{hyperref}
\usepackage{breakurl}
\usepackage{oneinchmargins}
\usepackage{tightenum}
\usepackage{wrapfig}
\usepackage{pifont}

\usepackage{enumitem}
\usepackage{listings}
\usepackage{latexsym}
\usepackage{adjustbox}
\usepackage{graphicx}
\usepackage{floatflt}
\usepackage{setspace}
\usepackage{graphicx}
\usepackage{algorithm}
\usepackage{amsmath}
\usepackage[small,compact]{titlesec}
\usepackage{titling}
%\usepackage[usenames]{color}
%\usepackage{algorithmic}
% \titlespacing*{\section}{0em}{-0ex}{-2ex}
% \titlespacing*{\subsection}{0em}{-0ex}{-2ex}
% \titlespacing*{\subsubsection}{0em}{-0ex}{-2ex}
%\setstretch{0.98}
%\usepackage[table]{xcolor}
%\usepackage{tabularx,booktabs}

\usepackage{xspace}
\usepackage{makecell}
\usepackage{caption}

\usepackage[normalem]{ulem}

\input{defs}
%\setstretch{1.2}

\sloppy
\input{macros}
%\newcommand{\ignore}[1]{}
%\input{remark}
%% Leave this on, so we can see them!!!
%$\remarktrue
%\remarkfalse

%\newcommand{\shortsec}{\vspace*{-0.2in}}
%\newcommand{\sparagraph}[1]{\vspace*{-0.2in}\paragraph{#1}}
%\newcommand{\sparagraph}[1]{\vspace*{-0.15in}\paragraph{#1}}

%\usepackage{draftwatermark}
%\SetWatermarkText{DO NOT DISTRIBUTE}
%\SetWatermarkScale{0.4}
\setlength{\columnsep}{0.33in}

\usepackage{xcolor}
\definecolor{commentgreen}{RGB}{2,112,10}
\definecolor{eminence}{RGB}{108,48,130}
\definecolor{weborange}{RGB}{255,165,0}
\definecolor{frenchplum}{RGB}{129,20,83}

\usepackage{listings}
\lstset {
    language=Python,
    frame=tb,
    tabsize=2,
    showstringspaces=false,
    %numbers=left,
    %upquote=true,
    commentstyle=\color{commentgreen},
    keywordstyle=\color{eminence},
    stringstyle=\color{red},
    basicstyle=\scriptsize\ttfamily, % basic font setting
    emph={int,char,double,float,unsigned,void,bool},
    emphstyle={\color{blue}},
    otherkeywords={Channel,read,write,write_async,flush,release},
    keywordstyle={\color{blue}},
    escapechar=\&,
    % keyword highlighting
    classoffset=1, % starting new class
    %otherkeywords={>,<,.,;,-,!,=,~},
    %morekeywords={>,<,.,;,-,!,=,~},
    %keywordstyle=\color{weborange},
    classoffset=0,
}

\usepackage{geometry}
\geometry{reset, letterpaper, height=9in, width=7in, hmarginratio=1:1, vmarginratio=1:1, marginparsep=0pt, marginparwidth=1.8cm, headheight=15pt}
% \usepackage{draftwatermark}
% \SetWatermarkText{Draft}
% \SetWatermarkScale{2}
% begin usenix styling
% \setlength{\textheight}{9.0in}
% \setlength{\columnsep}{0.33in}
% \setlength{\textwidth}{7.00in}

% \setlength{\topmargin}{0.0in}

% \setlength{\headheight}{0.0in}

% \setlength{\headsep}{0.0in}

% \addtolength{\oddsidemargin}{-0.25in}
% \addtolength{\evensidemargin}{-0.25in}

% end usenix styling

\begin{document}

% \pagestyle{plain}

% \if 0
\twocolumn[
 \begin{@twocolumnfalse}
 \begin{center}
 {\Large\bf Resource-Centric Serverless Computing}
 \end{center}
 \smallskip

 \bigskip
 \end{@twocolumnfalse}
 ]

% \fi

%\title{\Large\bf Resource-Centric Serverless Computing}

% \author{
% Zhiyuan Guo \qquad 
% Zachary Blanco\qquad
% Mohammad Shahrad\textsuperscript{*} \qquad
% Zerui Wei \\
% Bili Dong \qquad
% Jinmou Li \qquad
% Ishaan Pota\textsuperscript{$\mathsection$} \qquad
% Harry Xu\textsuperscript{$\mathsection$} \qquad
% Yiying Zhang \\
% }
% \date{\it{
% %\textsuperscript{\textdagger}
% UC San Diego \qquad
% \textsuperscript{*}University of British Columbia \qquad
% \textsuperscript{$\mathsection$}UC Los Angeles
% }}

%\maketitle

\thispagestyle{empty}

\input{appendix.tex}

\end{document}
